# Supplementary material for: Lorentz Reciprocal Theorem in Fluids with Odd Viscosity
Source: arXiv:2305.15379 ancillary file (2023-09-06)
Supplement: Supplementary file 1 [file supplemental_material.pdf]

# Lorentz Reciprocal Theorem in Fluids with Odd Viscosity
*Supplemental Material*

Yuto Hosaka,[1,*] Ramin Golestanian,[1,2,3,†] and Andrej Vilfan[1,4,‡]

[1] *Max Planck Institute for Dynamics and Self-Organization (MPI-DS), Am Fassberg 17, 37077 Göttingen, Germany*
[2] *Rudolf Peierls Centre for Theoretical Physics, University of Oxford, Oxford OX1 3PU, UK*
[3] *Institute for the Dynamics of Complex Systems, University of Göttingen, 37077 Göttingen, Germany*
[4] *Jožef Stefan Institute, 1000 Ljubljana, Slovenia*

## GENERALIZED LORENTZ RECIPROCAL THEOREM FOR A TWO-PHASE COMPRESSIBLE FLOW WITH ODD VISCOSITY

The Lorentz reciprocal theorem given in the main article is valid if the even (odd) viscosity tensor of the main problem has the same (opposite) sign as that of the auxiliary problem. Here we provide a more general form of the reciprocal theorem for a two-phase compressible flow with odd viscosity. Let the unhatted and hatted symbols represent the variables for any two arbitrary types of flows that satisfy the following equations:

$$\partial_j \sigma_{ij} + \mathfrak{f}_i = 0, \quad \partial_j \hat{\sigma}_{ij} + \hat{\mathfrak{f}}_i = 0, \tag{S1}$$

where $\sigma_{ij} = -p\delta_{ij} + \eta_{ijk\ell}\partial_\ell v_k$ and $\hat{\sigma}_{ij} = -\hat{p}\delta_{ij} + \hat{\eta}_{ijk\ell}\partial_\ell \hat{v}_k$ are the stress tensors with the pressure field $p$, the identity tensor $\delta_{ij}$, the viscosity tensor $\boldsymbol{\eta}$, the velocity field $\mathbf{v}$, and the arbitrary body force density $\mathfrak{f}$.

The inner product of $\mathbf{v}$ with the second expression in Eq. (S1) gives

$$\partial_j(\hat{\sigma}_{ij} v_i) + \hat{p}\partial_i v_i - \hat{\eta}_{k\ell ij}(\partial_\ell v_k)(\partial_j \hat{v}_i) + \hat{\mathfrak{f}}_i v_i = 0, \tag{S2}$$

and the equivalent expression with $\boldsymbol{\sigma}$ and $\hat{\mathbf{v}}$

$$\partial_j(\sigma_{ij} \hat{v}_i) + p\partial_i \hat{v}_i - \eta_{ijk\ell}(\partial_\ell v_k)(\partial_j \hat{v}_i) + \mathfrak{f}_i \hat{v}_i = 0. \tag{S3}$$

In general, the viscosity tensor can be decomposed into its symmetric and antisymmetric components with respect to swapping the indices $ij \leftrightarrow k\ell$, namely, $\boldsymbol{\eta} = \boldsymbol{\eta}^{\mathrm{e}} + \boldsymbol{\eta}^{\mathrm{o}}$, each of which satisfies

$$\eta^{\mathrm{e}}_{ijk\ell} = \eta^{\mathrm{e}}_{k\ell ij}, \quad \eta^{\mathrm{o}}_{ijk\ell} = -\eta^{\mathrm{o}}_{k\ell ij}. \tag{S4}$$

Based on this symmetry argument, we find from Eqs. (S2) and (S3)

$$\partial_j(\hat{\sigma}_{ij} v_i) + \hat{p}\partial_i v_i - (\hat{\eta}^{\mathrm{e}}_{ijk\ell} - \hat{\eta}^{\mathrm{o}}_{ijk\ell})(\partial_\ell v_k)(\partial_j \hat{v}_i) + \hat{\mathfrak{f}}_i v_i = 0, \tag{S5}$$

$$\partial_j(\sigma_{ij} \hat{v}_i) + p\partial_i \hat{v}_i - (\eta^{\mathrm{e}}_{ijk\ell} + \eta^{\mathrm{o}}_{ijk\ell})(\partial_\ell v_k)(\partial_j \hat{v}_i) + \mathfrak{f}_i \hat{v}_i = 0. \tag{S6}$$

If we allow for the linear relation between the two tensorial quantities, i.e., $\hat{\boldsymbol{\eta}}^{\mathrm{e}} - \hat{\boldsymbol{\eta}}^{\mathrm{o}} = c(\boldsymbol{\eta}^{\mathrm{e}} + \boldsymbol{\eta}^{\mathrm{o}})$ with a constant $c$ and subtract Eq. (S6) from Eq. (S5), we obtain

$$\partial_j(\hat{\sigma}_{ij} v_i) + \hat{p}\partial_i v_i + \hat{\mathfrak{f}}_i v_i = c[\partial_j(\sigma_{ij}\hat{v}_i) + p\partial_i \hat{v}_i + \mathfrak{f}_i \hat{v}_i]. \tag{S7}$$

Integrating over the fluid volume $\mathcal{V}$ and using the divergence theorem to obtain corresponding surface integrals over all bounding surfaces $\mathcal{S}$ [S1], the generalized reciprocal theorem is derived as

$$\int_{\mathcal{S}} dS\, \mathbf{v}\cdot\hat{\boldsymbol{\sigma}}\cdot\mathbf{n} - \int_{\mathcal{V}} dV\, (\hat{p}\nabla\cdot\mathbf{v} + \hat{\mathfrak{f}}\cdot\mathbf{v}) = c\left[\int_{\mathcal{S}} dS\, \hat{\mathbf{v}}\cdot\boldsymbol{\sigma}\cdot\mathbf{n} - \int_{\mathcal{V}} dV\, (p\nabla\cdot\hat{\mathbf{v}} + \mathfrak{f}\cdot\hat{\mathbf{v}})\right], \tag{S8}$$

where $\mathbf{n}$ is a surface normal pointing into the fluid. For incompressible fluids with $c = 1$ and without body forces, the Lorentz reciprocal theorem as derived in the main text is recovered.

## MOTION OF NO-SLIP AND PERFECT-SLIP SPHERE AND DISK IN THE ODD STOKES FLOW

In the following we show the derivations of flow fields around no-slip and perfect-slip spherical and disk-shaped bodies, needed to derive the active swimming velocity of a microswimmer in odd-viscous fluids.

### Green's functions for 3D odd flows

We begin by deriving Green's functions of 3D Stokes flows induced by a force density $\hat{\mathfrak{f}}$ acting on the fluid

$$\partial_j \hat{\sigma}_{ij} + \hat{\mathfrak{f}}_i = 0, \quad \partial_i \hat{v}_i = 0, \tag{S9}$$

where the stress tensor with odd viscosity is given by [S2]

$$\hat{\sigma}_{ij} = -\hat{p}\delta_{ij} + \hat{\eta}^{\rm e}(\partial_i \hat{v}_j + \partial_j \hat{v}_i) + \frac{\hat{\eta}^{\rm o}}{2}[\epsilon_{zik}(\partial_k \hat{v}_j + \partial_j \hat{v}_k) + \epsilon_{zjk}(\partial_i \hat{v}_k + \partial_k \hat{v}_i)]. \tag{S10}$$

In the above, $\hat{\mathbf{v}}$ is the velocity field, $\hat{p}$ is the pressure field, and $\hat{\eta}^{\rm e}$ and $\hat{\eta}^{\rm o}$ are the even (shear) and odd viscosities of the fluid, respectively, with $\delta_{ij}$ being the identity tensor and $\epsilon_{ijk}$ being the Levi-Civita tensor. The symbol $\hat{}$ denotes the quantities associated with the auxiliary problem to distinguish them from the main problems of active swimming. The specific form of Eq. (S9) reads

$$\hat{\eta}^{\rm e}\nabla^2 \hat{\mathbf{v}} - \frac{\hat{\eta}^{\rm o}}{2}\partial_z(\nabla \times \hat{\mathbf{v}}) - \nabla \hat{P} + \hat{\mathfrak{f}} = \mathbf{0}, \tag{S11}$$

where we have introduced the effective pressure $\hat{P} = \hat{p} - \hat{\eta}^{\rm o}(\nabla \times \hat{\mathbf{v}})_z$.

The Green's functions represent the response to a point force $\mathbf{A}$ acting locally at the origin, written in this form $\hat{\mathfrak{f}} = 8\pi\hat{\eta}^{\rm e}\mathbf{A}\delta(\mathbf{r})$, with the position vector $\mathbf{r} = (x, y, z)$. The resulting velocity, pressure, and stress fields can then be expressed with the following Green's functions [S3]

$$\hat{v}_i = G_{ij}A_j, \quad \hat{p} = \Pi_i A_i, \quad \hat{\sigma}_{ik} = T_{ijk}A_j, \tag{S12}$$

where $\mathbf{G}$ is the Stokeslet, and $\mathbf{\Pi}$ and $\mathbf{T}$ are the pressure vector and stress tensor associated with the Green's function.

To the first order in $\hat{\lambda} = \hat{\eta}^{\rm o}/\hat{\eta}^{\rm e}$, the Stokeslet for a 3D unbounded fluid with odd viscosity $\mathbf{G} = \mathbf{G}^{\rm e} + \mathbf{G}^{\rm o}$ has the two contributions

$$\mathbf{G}^{\rm e} = \frac{1}{r}\left(\mathbf{I} + \frac{\mathbf{rr}}{r^2}\right), \quad \mathbf{G}^{\rm o} = -\frac{\hat{\lambda}}{2r}\boldsymbol{\epsilon}\cdot\left(\mathbf{e}_z - \frac{z\mathbf{r}}{r^2}\right), \tag{S13}$$

with $r = |\mathbf{r}|$. Here $\mathbf{G}^{\rm e}$ is the classical Stokeslet without odd viscosity [see Eq. (2.2.8) in Ref. [S3]] and $\mathbf{G}^{\rm o}$ contains all corrections that are linear in $\hat{\lambda}$. Note that the Stokeslet $\mathbf{G}$ with a prefactor $1/(8\pi\hat{\eta}^{\rm e})$ is equivalent to Eq. (H6) in Ref. [S4] with $\eta_1^o = -2\eta_2^o = \hat{\eta}^{\rm o}$ and Eq. (20) in Ref. [S5] with $\mu_o = \hat{\eta}^{\rm o}/2$. Then the corresponding components of the (potential) source dipole $\mathbf{D} = \mathbf{D}^{\rm e} + \mathbf{D}^{\rm o}$ are given by

$$\mathbf{D}^{\rm e} = \frac{1}{2}\nabla^2\mathbf{G}^{\rm e} = \frac{1}{r^3}\left(\mathbf{I} - 3\frac{\mathbf{rr}}{r^2}\right), \quad \mathbf{D}^{\rm o} = \frac{1}{2}\nabla^2\mathbf{G}^{\rm o} = \frac{\hat{\lambda}}{2r^3}\boldsymbol{\epsilon}\cdot\left(\mathbf{e}_z - 3\frac{z\mathbf{r}}{r^2}\right), \tag{S14}$$

where $\mathbf{D}^{\rm e}$ with a minus sign is equivalent to Eq. (7.2.3) in Ref. [S3]. Noting that $\nabla \times \mathbf{D}^{\rm e} = \mathbf{0}, \nabla^2\mathbf{D}^{\rm e} = \mathbf{0}$, and $\nabla^2\mathbf{D}^{\rm o} = \mathbf{0}$, each source dipole independently satisfies the Stokes equation (S11) to the first order in $\hat{\lambda}$, with zero pressure ($\hat{p} = \hat{P} = 0$).

For the Stokeslet in Eq. (S13), the stress tensor is defined as

$$\begin{aligned} T_{ijk}^{\rm G^e} &= -(\Pi_j^{\rm G^e} + \hat{\eta}^{\rm o}\epsilon_{z\ell m}\partial_\ell G_{mj}^{\rm e})\delta_{ik} + \hat{\eta}^{\rm e}(\partial_i G_{kj}^{\rm e} + \partial_k G_{ij}^{\rm e}) + \frac{\hat{\eta}^{\rm o}}{2}[\epsilon_{zi\ell}(\partial_\ell G_{kj}^{\rm e} + \partial_k G_{\ell j}^{\rm e}) + \epsilon_{zk\ell}(\partial_i G_{\ell j}^{\rm e} + \partial_\ell G_{ij}^{\rm e})], \\ T_{ijk}^{\rm G^o} &= \hat{\eta}^{\rm e}(\partial_i G_{kj}^{\rm o} + \partial_k G_{ij}^{\rm o}), \end{aligned} \tag{S15}$$

where $\mathbf{\Pi}^{\rm G^e} = 2\hat{\eta}^{\rm e}\mathbf{r}/r^3$ is the pressure due to $\mathbf{G}^{\rm e}$ in Eq. (S13), while that due to $\mathbf{G}^{\rm o}$ in Eq. (S13) becomes zero. Inserting each Green's function in Eq. (S13) into Eq. (S15) yields

$$\begin{aligned} T_{ijk}^{\rm G^e} &= \frac{2\hat{\eta}^{\rm o}\epsilon_{z\ell j}r_\ell}{r^3}\delta_{ik} - \frac{6\hat{\eta}^{\rm e}r_j}{r^5}\left[r_i r_k + \hat{\lambda}\frac{r_\ell}{2}(\epsilon_{zi\ell}r_k + \epsilon_{zk\ell}r_i)\right], \\ T_{ijk}^{\rm G^o} &= \frac{\hat{\eta}^{\rm o}}{2r^3}\left[\epsilon_{ij\ell}r_\ell\left(\delta_{kz} - 3\frac{zr_k}{r^2}\right) + \epsilon_{kj\ell}r_\ell\left(\delta_{iz} - 3\frac{zr_i}{r^2}\right) + \epsilon_{zij}r_k + \epsilon_{zkj}r_i\right]. \end{aligned} \tag{S16}$$

Replacing $\mathbf{G}^{\mathrm{e}}$ with $\mathbf{D}^{\mathrm{e}}$ and $\mathbf{G}^{\mathrm{o}}$ with $\mathbf{D}^{\mathrm{o}}$ in Eq. (S15) and noting that the source dipole gives no pressure, we find

$$\begin{aligned} T_{ijk}^{\mathrm{D^e}} &= -\frac{6\hat{\eta}^{\mathrm{e}}}{r^5}\left[\delta_{kj}r_i + \delta_{ki}r_j + \delta_{ij}r_k - 5\frac{r_ir_jr_k}{r^2} + \frac{\hat{\lambda}}{2}\left[\epsilon_{zij}r_k + \epsilon_{zkj}r_i + \epsilon_{zi\ell}r_\ell\left(\delta_{kj} - 5\frac{r_kr_j}{r^2}\right) + \epsilon_{zk\ell}r_\ell\left(\delta_{ij} - 5\frac{r_ir_j}{r^2}\right)\right]\right], \\ T_{ijk}^{\mathrm{D^o}} &= -\frac{3\hat{\eta}^{\mathrm{o}}}{2r^5}\left[\epsilon_{zij}r_k + \epsilon_{zkj}r_i + \epsilon_{ijm}r_m\left(\delta_{zk} - 5\frac{zr_k}{r^2}\right) + \epsilon_{kjm}r_m\left(\delta_{zi} - 5\frac{zr_i}{r^2}\right)\right]. \end{aligned} \tag{S17}$$

## Green's functions for 2D odd flows

In a 2D flow, applying the incompressibility condition simplifies Eq. (S10) to

$$\hat{\sigma}_{ij} = -\hat{P}\delta_{ij} + \hat{\eta}^{\mathrm{e}}(\partial_i\hat{v}_j + \partial_j\hat{v}_i) + 2\hat{\eta}^{\mathrm{o}}\epsilon_{zjk}\partial_k\hat{v}_i, \tag{S18}$$

with $\hat{P} = \hat{p} - \hat{\eta}^{\mathrm{o}}(\nabla\times\hat{\mathbf{v}})_z$ being the effective pressure as before. To derive the Green's function, we consider Stokes flows induced by a 2D force density $\hat{\mathbf{f}}$ acting on the fluid, i.e., $\partial_j\hat{\sigma}_{ij} + \hat{\mathrm{f}}_i = 0$. From Eq. (S18), the 2D Stokes equation is obtained as

$$\hat{\eta}^{\mathrm{e}}\nabla^2\hat{\mathbf{v}} - \nabla\hat{P} + \hat{\mathbf{f}} = \mathbf{0}. \tag{S19}$$

Consider a point force $\mathbf{B}$ acting locally at the origin, written in this form $\hat{\mathbf{f}} = 4\pi\hat{\eta}^{\mathrm{e}}\mathbf{B}\delta(\boldsymbol{\rho})$, with the position vector $\boldsymbol{\rho} = (x, y)$. Then, the solution of the 2D Stokes equation (S19) can be represented in terms of Green's functions for the velocity, effective pressure, and stress fields [S3]

$$\hat{v}_i = g_{ij}B_j, \quad \hat{P} = \Pi_i^{\mathrm{g}}B_i, \quad \hat{\sigma}_{ik} = T_{ijk}^{\mathrm{g}}B_j. \tag{S20}$$

The corresponding Stokeslet is the same as in classical fluids without odd viscosity, given by [see Eq. (2.6.17) in Ref. [S3]]

$$\mathbf{g} = -\ln\left(\frac{\rho}{a}\right)\mathbf{I} + \frac{\boldsymbol{\rho}\boldsymbol{\rho}}{\rho^2}, \tag{S21}$$

where $\rho = |\boldsymbol{\rho}|$ and $a$ is the cutoff length, which in the case of the disk geometry is equal to the radius. The corresponding Green's function for the pressure is $\boldsymbol{\Pi}^{\mathrm{g}} = 2\hat{\eta}^{\mathrm{e}}\boldsymbol{\rho}/\rho^2$.

The flow due to a (potential) source dipole is also identical to that without odd viscosity [see Eq. (3.5.2) in Ref. [S3]]

$$\mathbf{d} = \frac{1}{2}\nabla^2\mathbf{g} = \frac{1}{\rho^2}\left(\mathbf{I} - 2\frac{\boldsymbol{\rho}\boldsymbol{\rho}}{\rho^2}\right). \tag{S22}$$

Because of $\nabla^2\mathbf{d} = \mathbf{0}$, the source dipole does not contribute to the effective pressure $\hat{P}$, while $\nabla\times\mathbf{d} = \mathbf{0}$ means that there is no pressure $\hat{p}$ due to the source dipole. In total, the source dipole gives no pressure $\hat{p} = \hat{P} = 0$.

For the Stokeslet and source dipole, the stress tensor is defined as

$$T_{ijk}^{\mathrm{g}} = -\delta_{ik}\Pi_j^{\mathrm{g}} + \hat{\eta}^{\mathrm{e}}(\partial_i g_{kj} + \partial_k g_{ij}) + 2\hat{\eta}^{\mathrm{o}}\epsilon_{zk\ell}\partial_\ell g_{ij}, \quad T_{ijk}^{\mathrm{d}} = \hat{\eta}^{\mathrm{e}}(\partial_i d_{kj} + \partial_k d_{ij}) + 2\hat{\eta}^{\mathrm{o}}\epsilon_{zk\ell}\partial_\ell d_{ij}. \tag{S23}$$

Inserting the Green's functions of Eqs. (S21) and (S22) into the above expressions yields

$$\begin{aligned} T_{ijk}^{\mathrm{g}} &= -\frac{2\hat{\eta}^{\mathrm{e}}}{\rho^2}\left[2(\delta_{k\ell} + \hat{\lambda}\epsilon_{zk\ell})\frac{\rho_i\rho_j\rho_\ell}{\rho^2} + \hat{\lambda}\epsilon_{zk\ell}\left(\delta_{ij}\rho_\ell - \delta_{i\ell}\rho_j - \delta_{j\ell}\rho_i\right)\right], \\ T_{ijk}^{\mathrm{d}} &= -\frac{4\hat{\eta}^{\mathrm{e}}}{\rho^4}(\delta_{k\ell} + \hat{\lambda}\epsilon_{zk\ell})\left(\delta_{ij}\rho_\ell + \delta_{i\ell}\rho_j + \delta_{j\ell}\rho_i - 4\frac{\rho_i\rho_j\rho_\ell}{\rho^2}\right). \end{aligned} \tag{S24}$$

Note here that the above solutions are exact for any value of the ratio $\hat{\lambda} = \hat{\eta}^{\mathrm{e}}/\hat{\eta}^{\mathrm{o}}$, unlike 3D flows where $\hat{\lambda} \ll 1$ is assumed.

### Boundary conditions

We now consider the flow around a body moving with the velocity $\hat{\mathbf{V}}$. In the co-moving frame, the boundary conditions for this motion take the form

$$\hat{\mathbf{v}} = -\hat{\mathbf{V}}, \quad r \to \infty \tag{S25}$$

$$\mathbf{n} \cdot \hat{\mathbf{v}} = 0, \quad \mathbf{r} \in \mathcal{S} \tag{S26}$$

where $\mathbf{n}$ is a unit vector normal to the body surface, and $\mathcal{S}$ denotes the surface of the particle. Equation (S25) indicates that the effect of the particle must vanish in the far-field flow, and Eq. (S26) imposes the kinematic (or impermeability) boundary condition at the surface. By definition, a no-slip body has no surface velocity, while a perfect-slip body has no tangential traction. These conditions are, respectively, given by

$$\hat{\mathbf{v}}_{\mathrm{NS}} = \mathbf{0}, \quad \mathbf{r} \in \mathcal{S} \tag{S27}$$

$$(\mathbf{I} - \mathbf{nn}) \cdot \hat{\boldsymbol{\sigma}}_{\mathrm{PS}} \cdot \mathbf{n} = \mathbf{0}. \quad \mathbf{r} \in \mathcal{S} \tag{S28}$$

### No-slip sphere

To describe the flow around a no-slip sphere fixed at the origin $\mathbf{r} = \mathbf{0}$ to the first order in $\hat{\lambda} = \hat{\eta}^{\mathrm{o}}/\hat{\eta}^{\mathrm{e}}$, we use a superposition of a Stokeslet and source dipole as an ansatz

$$\hat{\mathbf{v}}_{\mathrm{NS}} = -\hat{\mathbf{V}} + \mathbf{G} \cdot \mathbf{A}_1 + \mathbf{D} \cdot \mathbf{A}_2 + \mathbf{G}^{\mathrm{e}} \cdot \mathbf{A}_3 + \mathbf{D}^{\mathrm{e}} \cdot \mathbf{A}_4, \tag{S29}$$

where $\mathbf{A}_1, \dots, \mathbf{A}_4$ are unknown coefficient vectors that will be determined from the boundary condition given in Eq. (S27). We then find

$$\mathbf{A}_1 = \frac{3a}{4}\,\hat{\mathbf{V}}, \quad \mathbf{A}_2 = \frac{a^3}{4}\,\hat{\mathbf{V}}, \quad \mathbf{A}_3 = -\hat{\lambda}\,\frac{3a}{16}\,\mathbf{e}_z \times \hat{\mathbf{V}}, \quad \mathbf{A}_4 = -\hat{\lambda}\,\frac{a^3}{16}\,\mathbf{e}_z \times \hat{\mathbf{V}}. \tag{S30}$$

The stress tensor can be expressed with the corresponding Green's functions, as defined in Eq. (S12):

$$\hat{\sigma}_{\mathrm{NS},ik} = T^{\mathrm{G^e}}_{ijk}(A_{1,j} + A_{3,j}) + T^{\mathrm{G^o}}_{ijk} A_{1,j} + T^{\mathrm{D^e}}_{ijk}(A_{2,j} + A_{4,j}) + T^{\mathrm{D^o}}_{ijk} A_{2,j}. \tag{S31}$$

By using the explicit expressions from Eqs. (S16) and (S17), we obtain the traction at the surface $\hat{\mathbf{f}}_{\mathrm{NS}} = \hat{\boldsymbol{\sigma}}_{\mathrm{NS}} \cdot \mathbf{n}$

$$\hat{\mathbf{f}}_{\mathrm{NS}} = -\frac{3\hat{\eta}^{\mathrm{e}}}{2a}\left(\hat{\mathbf{V}} - \frac{\hat{\lambda}}{4}\mathbf{e}_z \times \hat{\mathbf{V}}\right), \tag{S32}$$

and the total force is

$$\hat{\mathbf{F}}_{\mathrm{NS}} = -6\pi\hat{\eta}^{\mathrm{e}} a\left(\hat{\mathbf{V}} - \frac{\hat{\lambda}}{4}\mathbf{e}_z \times \hat{\mathbf{V}}\right). \tag{S33}$$

### Perfect-slip sphere

For the velocity field around a perfect-slip sphere ("bubble"), we use a superposition of a Stokeslet and a source dipole as an ansatz

$$\hat{\mathbf{v}}_{\mathrm{PS}} = -\hat{\mathbf{V}} + \mathbf{G} \cdot \mathbf{A}'_1 + \mathbf{D}^{\mathrm{e}} \cdot \mathbf{A}'_2 + \mathbf{D}^{\mathrm{o}} \cdot \mathbf{A}'_3. \tag{S34}$$

The stress tensor is given by an equivalent superposition of Green's functions that can be found in Eqs. (S16) and (S17):

$$\hat{\sigma}_{\mathrm{PS},ik} = (T^{\mathrm{G^e}}_{ijk} + T^{\mathrm{G^o}}_{ijk}) A'_{1,j} + T^{\mathrm{D^e}}_{ijk} A'_{2,j} + T^{\mathrm{D^o}}_{ijk} A'_{3,j}. \tag{S35}$$

Imposing the boundary conditions of zero radial velocity (S26) and zero tangential traction (S28), we find

$$\mathbf{A}'_1 = \frac{a}{2}\,\hat{\mathbf{V}}, \quad \mathbf{A}'_2 = \hat{\lambda}\,\frac{a^3}{6}\,\mathbf{e}_z \times \hat{\mathbf{V}}, \quad \mathbf{A}'_3 = -\frac{a^3}{6}\,\hat{\mathbf{V}}. \tag{S36}$$

The flow velocity (S34) on the surface of the sphere then evaluates to

$$\hat{\mathbf{v}}_{\mathrm{PS}}^{\parallel} = \frac{1}{2}\left[(\mathbf{nn}-\mathbf{I})\cdot(\hat{\mathbf{V}}-\hat{\lambda}\mathbf{e}_z\times\hat{\mathbf{V}})-\hat{\lambda}\mathbf{e}_z\cdot\mathbf{nn}\times\hat{\mathbf{V}}\right], \tag{S37}$$

and the force is found as

$$\hat{\mathbf{F}}_{\mathrm{PS}} = -4\pi\hat{\eta}^{\mathrm{e}}a\hat{\mathbf{V}}. \tag{S38}$$

## Stokes paradox in 2D flows

For a 2D fluid at low Reynolds number, there is no solution of the creeping flow that vanishes at the perimeter of a disk and remains finite at infinity because the velocity diverges [S6]. The problem is therefore ill-posed in the laboratory frame. This is known as the Stokes paradox that originates from the constraint of momentum conservation in a purely 2D system. However, it is possible to obtain solutions in the co-moving frame. Although the 2D flow field at large distances still diverges, it is possible to determine a relationship between the velocity in the vicinity of the disk and the force acting on it [S7]. In addition, it is known that the relation between the total force and the traction at the disk is well-defined [S8]. Self-propelled swimmers in 2D flows are force-free and therefore not affected by the Stokes paradox. In the following, we obtain the relation between the force and the traction for a no-slip disk. Subsequently, the relationship between the force and the local velocity at the disk perimeter is obtained for a perfect-slip disk.

## No-slip disk

For the flow field around a no-slip disk, we use a superposition of a Stokeslet and source dipole as an ansatz

$$\hat{\mathbf{v}}_{\mathrm{NS}} = \mathbf{B}_0 + \mathbf{g}\cdot\mathbf{B}_1 + \mathbf{d}\cdot\mathbf{B}_2. \tag{S39}$$

From the no-slip boundary condition (S27), we determine

$$\mathbf{B}_0 = -\frac{1}{2}\mathbf{B}_1 = -\frac{1}{a^2}\mathbf{B}_2. \tag{S40}$$

The stress tensor can be expressed with the Green's functions defined in Eq. (S24) as

$$\hat{\sigma}_{\mathrm{NS},ik} = T^{\mathrm{g}}_{ijk}B_{1,j} + T^{\mathrm{d}}_{ijk}B_{2,j}. \tag{S41}$$

The traction $\hat{\mathbf{f}}_{\mathrm{NS}} = \hat{\boldsymbol{\sigma}}_{\mathrm{NS}}\cdot\mathbf{n}$ and force acting on the disk perimeter become

$$\hat{\mathbf{f}}_{\mathrm{NS}} = -\frac{2\hat{\eta}^{\mathrm{e}}}{a}\mathbf{B}_1, \quad \hat{\mathbf{F}}_{\mathrm{NS}} = -4\pi\hat{\eta}^{\mathrm{e}}\mathbf{B}_1. \tag{S42}$$

The force is independent of the odd viscosity as long as the boundary conditions include the velocity field alone [S9].

## Perfect-slip disk

To find the flow around a perfect-slip disk, we use the same singularities as those of the no-slip case

$$\hat{\mathbf{v}}_{\mathrm{PS}} = (b_1'\mathbf{I}+\mathbf{g})\cdot\mathbf{B}_1' + (b_2'\mathbf{I}+\mathbf{d})\cdot\mathbf{B}_2'. \tag{S43}$$

We split the constant velocity in two parts and require that each term satisfies the zero normal velocity boundary condition (S26) on its own. This is the case with $b_1' = -1$ and $b_2' = 1/a^2$. The stress tensor can be expressed with the Green's functions defined in Eq. (S24) as

$$\hat{\sigma}_{\mathrm{PS},ik} = T^{\mathrm{g}}_{ijk}B'_{1,j} + T^{\mathrm{d}}_{ijk}B'_{2,j}. \tag{S44}$$

By evaluating it at the disk perimeter, we obtain the tangential component of the traction

$$(\mathbf{I}-\mathbf{nn})\cdot\hat{\boldsymbol{\sigma}}_{\mathrm{PS}}\cdot\mathbf{n} = -\frac{4\hat{\eta}^{\mathrm{e}}}{a^3}(\mathbf{I}-\mathbf{nn})\cdot\mathbf{B}_2' + \frac{2\hat{\eta}^{\mathrm{o}}}{a}\mathbf{n}\cdot\left(\mathbf{B}_1' - \frac{2}{a^2}\mathbf{B}_2'\right)\mathbf{e}_z\times\mathbf{n}. \tag{S45}$$

The perfect-slip boundary condition (S28) requires that the tangential traction vanishes, which gives the conditions

$$\hat{\eta}^{\mathrm{o}}a^2B_{1,y}' + 2\hat{\eta}^{\mathrm{e}}B_{2,x}' - 2\hat{\eta}^{\mathrm{o}}B_{2,y}' = 0, \quad \hat{\eta}^{\mathrm{o}}a^2B_{1,x}' - 2\hat{\eta}^{\mathrm{e}}B_{2,y}' - 2\hat{\eta}^{\mathrm{o}}B_{2,x}' = 0. \tag{S46}$$

In vector notation, their solution for an arbitrary value of $\hat{\lambda} = \hat{\eta}^{\mathrm{o}}/\hat{\eta}^{\mathrm{e}}$ reads

$$\mathbf{B}_2' = \frac{a^2}{2}\frac{\hat{\lambda}}{1+\hat{\lambda}^2}\left(\mathbf{e}_z\times\mathbf{B}_1' + \hat{\lambda}\mathbf{B}_1'\right). \tag{S47}$$

The total force is again determined by the magnitude of the Stokeslet as

$$\hat{\mathbf{F}}_{\mathrm{PS}} = -4\pi\hat{\eta}^{\mathrm{e}}\mathbf{B}_1'. \tag{S48}$$

## FLOW FIELD OF A 2D FORCE-PRESCRIBED SWIMMER

In Fig. 2(b), we plot the streamlines in the co-moving frame of a flow induced by a force-prescribed swimmer of radius $a$ for $\lambda = \eta^{\mathrm{o}}/\eta^{\mathrm{e}} = 1$. We impose the boundary conditions of zero radial velocity $\mathbf{n}\cdot\mathbf{v}_{\mathrm{A}} = 0$ [see also Eq. (S26)] and prescribed tangential traction given by $f_{\mathrm{A}}^{||} = -f_0\sin\phi$ on the swimmer perimeter. From the force-free condition of the swimmer ($\mathbf{F}_{\mathrm{A}} = \mathbf{0}$), the resulting velocity field can be expressed solely with the 2D source dipole in Eq. (S22) and has the form

$$\mathbf{v}_{\mathrm{A}}(x,y) = \frac{af_0}{4\eta^{\mathrm{e}}}\frac{1}{1+\lambda^2}\left[\mathbf{I} + \frac{a^2}{\rho^2}\left(\mathbf{I} - 2\frac{\boldsymbol{\rho}\boldsymbol{\rho}}{\rho^2}\right)\right]\cdot(-\mathbf{e}_x + \lambda\mathbf{e}_y). \tag{S49}$$

## SURFACE PROFILES OF VELOCITY- AND FORCE-PRESCRIBED SWIMMERS IN FIG. 3

| | | |
|---|---|---|
| (a) $\mathbf{v}_{\mathrm{A}} = -v_0(\mathbf{I}-\mathbf{nn})\cdot\mathbf{e}_z$ | (b) $\mathbf{v}_{\mathrm{A}} = -v_0(\mathbf{I}-\mathbf{nn})\cdot\mathbf{e}_x$ | (c) $\mathbf{v}_{\mathrm{A}} = v_0\sin(2\theta)\mathbf{e}_\phi$ |
| (d) $\mathbf{f}_{\mathrm{A}}^{||} = f_0(\mathbf{I}-\mathbf{nn})\cdot\mathbf{e}_z$ | (e) $\mathbf{f}_{\mathrm{A}}^{||} = f_0(\mathbf{I}-\mathbf{nn})\cdot\mathbf{e}_x$ | (f) $\mathbf{f}_{\mathrm{A}}^{||} = f_0\sin(2\theta)\mathbf{e}_\phi$ |

* yuto.hosaka@ds.mpg.de
† ramin.golestanian@ds.mpg.de
‡ andrej.vilfan@ds.mpg.de

[S1] H. Masoud and H. A. Stone, The reciprocal theorem in fluid dynamics and transport phenomena, J. Fluid Mech. **879**, 1 (2019).
[S2] T. Markovich and T. C. Lubensky, Odd viscosity in active matter: Microscopic origin and 3D effects, Phys. Rev. Lett. **127**, 048001 (2021).
[S3] C. Pozrikidis, *Boundary Integral and Singularity Methods for Linearized Viscous Flow* (Cambridge University Press, Cambridge, 1992).
[S4] T. Khain, C. Scheibner, M. Fruchart, and V. Vitelli, Stokes flows in three-dimensional fluids with odd and parity-violating viscosities, J. Fluid Mech. **934**, A23 (2022).
[S5] H. Yuan and M. Olvera de la Cruz, Stokesian dynamics with odd viscosity, Phys. Rev. Fluids **8**, 054101 (2023).
[S6] J. Happel and H. Brenner, *Low Reynolds Number Hydrodynamics* (Springer Netherlands, 1983).
[S7] D. Hickey, A. Vilfan, and R. Golestanian, Ciliary chemosensitivity is enhanced by cilium geometry and motility, Elife **10**, e66322 (2021).
[S8] G. J. Elfring, A note on the reciprocal theorem for the swimming of simple bodies, Phys. Fluids **27**, 023101 (2015).
[S9] S. Ganeshan and A. G. Abanov, Odd viscosity in two-dimensional incompressible fluids, Phys. Rev. Fluids **2**, 094101 (2017).
